# Supplementary material for: Geometry-Aware Metric Learning for Cross-Lingual Few-Shot Sign Language Recognition on Static Hand Keypoints
Source: arXiv:2603.09213 source file (2026-03-10)
Supplement: Supplementary file 1 [file X_suppl.tex]

\clearpage
\setcounter{page}{1}
\maketitlesupplementary

\section{Supplementary Material}
\label{sec:supplementary}
This supplementary is compiled together with the main paper, which means:
\begin{itemize}
\item The supplementary can back-reference sections of the main paper---for example, the introduction (\cref{sec:intro}) or the invariance proof (\cref{eq:invariance}).
\item The main paper can forward-reference specific supplementary content (e.g., additional experiments or derivations).
\item When submitted to arXiv, the supplementary is automatically included at the end of the document.
\end{itemize}
To extract the supplementary pages from the main PDF, standard tools such as \href{https://support.apple.com/en-ca/guide/preview/prvw11793/mac#:~:text=Delete%20a%20page%20from%20a,or%20choose%20Edit%20%3E%20Delete).}{Preview (macOS)}, \href{https://www.adobe.com/acrobat/how-to/delete-pages-from-pdf.html#:~:text=Choose%20%E2%80%9CTools%E2%80%9D%20%3E%20%E2%80%9COrganize,or%20pages%20from%20the%20file.}{Adobe Acrobat}, or \href{https://superuser.com/questions/517986/is-it-possible-to-delete-some-pages-of-a-pdf-document}{command-line utilities} can be used.
